# Supplementary material for: Long-lived neighbors determine the rheological response of glasses
Source: arXiv:1612.00376 ancillary file (2016-12-01)
Supplement: Supplementary file 1 [file Laurati_yielding_accepted-SM.pdf]

# Supplemental Material

## Long-lived neighbors determine the rheological response of glasses

M. Laurati[1,2], P. Maßhoff[1], K. J. Mutch[1], S. U. Egelhaaf[1], and A. Zaccone[3]
[1] *Condensed Matter Physics Laboratory, Heinrich Heine University, 40225 Düsseldorf, Germany*
[2] *División de Ciencias e Ingeniería, Universidad de Guanajuato, León 37150, Mexico and*
[3] *Department of Chemical Engineering and Biotechnology, and Cavendish Laboratory, University of Cambridge, Cambridge CB2 3RA, UK*
(Dated: November 26, 2016)

### Experimental details

We investigated concentrated amorphous dispersions of polymethylmethacrylate (PMMA) hard-sphere like particles [1] with volume fractions $0.565 \le \phi \le 0.600$ [2], i.e. volume fractions around the colloidal glass transition ($\phi_{\rm g} \approx 0.58$) [3]. The samples contained either small spheres (radius $R_1 = 150$ nm, polydispersity $\sigma_{\rm R,1} \approx 12\%$) in a mixture of cis- and trans-decalin or large spheres ($R_2 = 780$ nm, $\sigma_{\rm R,2} \approx 6\%$) fluorescently labelled with 7-nitrobenzo-2-oxa-1,3-diazole-methylmethacrylate (NBD) in a mixture of cis-decalin and cycloheptyl bromide that closely matches their density and refractive index, and with 4 mM tetrabutylammoniumchloride to screen electrostatic interactions [4]. The solvent mixtures have a viscosity $\eta_{\rm s} \approx 3.6$ mPa s and 2.6 mPa s, respectively.

Start-up shear experiments were performed using a stress-controlled rheometer (TA Instruments, DHR3) for dispersions of the small particles, and a strain-controlled rheometer (TA Instruments, ARES-G2) for the large particles, with cone-plate geometries of 50 mm diameter and an angle of 0.5° and 2°, respectively. In the microscopy experiments, we used a home-built shear cell (described in [5]). It consists of two parallel glass plates driven by a piezo actuator. The geometries were coated with polydisperse PMMA particles to avoid wall slip [6]. Both, the shear rate and absence of slip were checked by confocal microscopy [7]. Loading and history effects were reduced by a rejuvenation procedure before starting each measurement. This consisted of applying typically 10 large amplitude oscillations (at a strain in excess of 100%) at a frequency below 0.1 Hz, and subsequently waiting for 600 s before the experiment is started.

Image stacks were acquired between 15 and 25 $\mu$m from the lower cover slip using a confocal microscope (Visitech, VT-Eye) mounted on an inverted microscope (Nikon, Ti-U with a Plan Apo VC 100× objective with NA=1.40). The stacks of 512×512×50 pixels correspond to $51 \times 51 \times 10\,\mu\text{m}^3$, contain ∼8500 particles and were acquired in $\Delta t = 1.83$ s. From one series of confocal images, particle coordinates and trajectories were extracted using standard routines and then refined [8, 9].

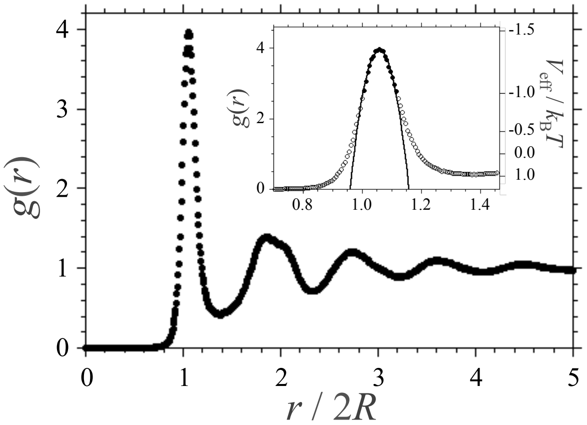


FIG. SM-1. Radial distribution function $g(r)$ as determined by confocal microscopy. (Inset) First maximum of $g(r)$ and corresponding pair potential of mean force $V_{\rm eff}(r)$. The line represents a quadratic fit to the first peak taking into account the data represented as filled circles.

### Effective spring constant

The effective (entropic) spring constant, $\kappa = [{\rm d}^2 V_{\rm eff}/{\rm d}r^2]_{r=r_{\rm m}}$ is related to the curvature of the minimum of the pair potential of mean force, $V_{\rm eff}(r)$, which is located at $r_{\rm m}$. The pair potential of mean force also takes into account the effects of all other particles on a particular pair of neighbors and is related to the radial distribution function $g(r)$ by $V_{\rm eff}(r) = -k_{\rm B}T \ln g(r)$ [10]. Thus, the spring constant $\kappa$ can be determined through the curvature of the first maximum of the radial distribution function $g(r)$ by

$$\kappa = \frac{{\rm d}^2 V_{\rm eff}}{{\rm d}r^2}(r_{\rm m}) = -k_{\rm B}T \left[ \frac{g''(r_{\rm m})}{g(r_{\rm m})} - \left( \frac{g'(r_{\rm m})}{g(r_{\rm m})} \right)^2 \right] , \quad \text{(SM-1)}$$

where $r_{\rm m}$ is the position of the first maximum of $g(r)$ and the second term vanishes since $g'(r_{\rm m}) = 0$ at the maximum. A quadratic fit to the first peak of $g(r)$ yields $\kappa = 50.2\, k_{\rm B}T/R_2^2$ for the present system (Fig. SM-1). This value is consistent with a theoretical prediction [11].

As mentioned in the main manuscript, the value of $\kappa$ can also be determined from the initial slope of the elastic stress $\sigma_{\rm el}(\gamma)$ according to

$$\kappa = \frac{5\pi R_2}{\phi\,(n_0{-}6)}\, G \qquad \text{(SM-2)}$$

where $R_2 = 780$ nm is the particle radius and $\phi = 0.565$ the volume fraction. The initial mean number of long-lived nearest neighbors $n_0 = 10.7$ and the shear modulus $G = [\partial\sigma_{\rm tot}(\gamma)/\partial\gamma]_{\gamma\to 0} \approx [\partial\sigma_{\rm el}(\gamma)/\partial\gamma]_{\gamma\to 0} = 8.41\, k_{\rm B}T/R_2^3$, exploiting that $\sigma_{\rm el} \approx \sigma_{\rm tot}$ for small $\gamma$. The rheological measurements (Fig. 3a) suggest $\kappa = 49.5\, k_{\rm B}T/R_2^2$, which agrees very well with the value determined through $g(r)$ obtained by confocal microscopy.

## Fit procedure and values of the fixed and fitted parameters

We derived the transient total stress (Eqs. 5, 6)

$$\sigma_{\rm tot}(\gamma) = \frac{\kappa\phi}{10\pi R}\left\{2\,(n_0{-}6)\,\gamma\left(1{-}\left(\frac{\gamma}{\xi}\right)^2\right)e^{-\left(\frac{\gamma}{\xi}\right)^2} - 3c\gamma^2\right\} + \dot\gamma\eta\left\{1{-}e^{-\left(\frac{\gamma}{\dot\gamma\tau_{\rm v}}\right)^\beta}\right\} \qquad \text{(SM-3)}$$

where the first term represents the affine and non-affine elastic stresses and the second term the viscous contribution. The theory describing the non-affine elastic stress is no longer valid once the system behaves fluid-like, i.e. beyond yielding. This is responsible for the elastic part decaying to minus infinity, $\sigma_{\rm el}(\gamma{\to}\infty) \to -\infty$ (for $c \neq 0$), which is unphysical. Therefore, $\sigma_{\rm el}$ is assumed to attain a constant value beyond the characteristic strain $\xi$ of the exponential decay, i.e. $\sigma_{\rm el}(\gamma{\geq}\xi) = \sigma_{\rm el}(\xi)$. Since for the present system $c = 0$, this implies $\sigma_{\rm el}(\gamma{\geq}\xi) = 0$. Although this avoids the unphysical behavior for $\gamma > \xi$, the abrupt change to the constant value $\sigma_{\rm el}(\xi)$ is still unphysical and leads to a kink of $\sigma_{\rm el}(\gamma)$ at $\gamma = \xi$ (Fig. SM-2a, dotted line). Nevertheless, the effect of the abrupt change is limited to a much smaller region, $\gamma \approx \xi$, as compared to $\gamma \gtrsim \xi$. The abrupt change could be avoided by an empirical interpolation. However, this would introduce free parameters, which we prefer to avoid.

Most of the parameters in Eq. SM-3 are known and hence are fixed. The particle radius $R$ and volume fraction $\phi$ are given through the sample composition and the shear rate $\dot\gamma$ through the experimental conditions. In the case of the large particles, confocal microscopy allows us to determine the initial mean number of long-lived nearest neighbors $n_0 = 10.7$, the first-order correction term $c = 0$, the characteristic decay parameter $\xi = 0.31$ and the spring constant $\kappa \approx 50\, k_{\rm B}T/R_2^2$, where the latter agrees with the value determined from the initial slope of $\sigma_{\rm tot}(\gamma)$. Moreover, the viscosity $\eta = 2.6$ Pa s $= 10^3\,\eta_{\rm s}$ can be determined from the steady-state value $\sigma_{\rm tot}(\gamma{\to}\infty) \approx \sigma_{\rm el}(\gamma{\to}\infty) = \dot\gamma\eta$. This leaves

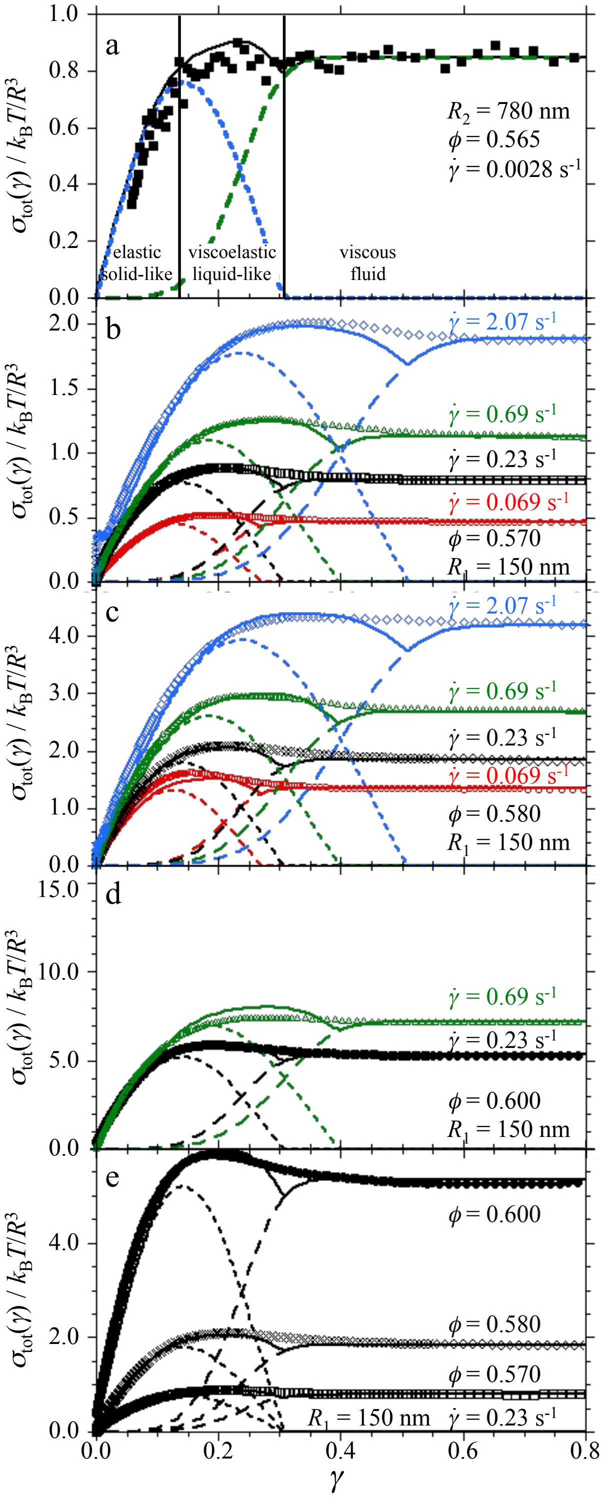


FIG. SM-2. (Color online) Normalized transient total stress $\sigma_{\rm tot}(\gamma)/(k_{\rm B}T/R^3)$ as a function of strain $\gamma = \dot\gamma t$ during start-up for (a) large spheres and (b–e) small spheres with (b–d) different shear rates $\dot\gamma$ for three volume fractions $\phi$ and (e) different $\phi$ for one $\dot\gamma$ with $\dot\gamma$, $\phi$ and the particle radius $R$ as indicated. Symbols represent experimental data, solid lines fits (Eq. SM-3), dotted and dashed lines the elastic, $\sigma_{\rm el}(\dot\gamma)$ (Eq. 5), and viscous, $\sigma_{\rm disc}(\dot\gamma)$ (Eq. 6), contributions, respectively. The different regimes are indicated in (a).

TABLE SM-1. Fixed and fitted parameters for the sample containing large particles and the sample containing small particles under the corresponding conditions, i.e. similar volume fraction $\phi$ and Peclet number $Pe_0$. See text for details.

| parameter | large particles | | small particles | |
|---|---|---|---|---|
| radius $R$ | 780 nm | fixed | 150 nm | fixed |
| volume fraction $\phi$ | 0.565 | fixed | 0.570 | fixed |
| shear rate $\dot{\gamma}$ | 0.0028 $\mathrm{s}^{-1}$ | fixed | 0.23 $\mathrm{s}^{-1}$ | fixed |
| long-lived neighbors $n_0$ | 10.7 | fixed | 10.7 | fixed |
| first-order term $c$ | 0 | fixed | 0 | fixed |
| decay parameter $\xi$ | 0.31 | fixed | 0.31 | fixed |
| spring constant $\kappa$ | $50\,k_\mathrm{B}T/R_2^2$ | fixed | $50\,k_\mathrm{B}T/R_1^2$ | fixed |
| viscosity $\eta$ | $1.0{\times}10^3\,\eta_\mathrm{s}$ | fixed | $1.1{\times}10^3\,\eta_\mathrm{s}$ | fixed |
| viscous time scale $\tau_\mathrm{v}$ | **$0.25/\dot{\gamma}$** | **fitted** | $0.25/\dot{\gamma}$ | fixed |
| stretching exponent $\beta$ | **4.6** | **fitted** | 4.6 | fixed |

the viscous time scale $\tau_\mathrm{v}$ and the stretching exponent $\beta$ as the only free parameters. As discussed in the main part of the manuscript, the model (Eq. SM-3) describes the experimentally determined $\sigma_\mathrm{tot}(\gamma)$ (Fig. 3a and SM-2a) very well. It yields $\beta = 4.6$, consistent with the expectation that it should be considerably larger than 2. Moreover, the fitted value $\tau_\mathrm{v} = 89$ s $= 16\,\tau_\mathrm{B}$ with the Brownian time $\tau_\mathrm{B} = 6\pi\eta_\mathrm{s}R_2^3/(k_\mathrm{B}T) = 5.7$ s is comparable to the value predicted through Maxwell's expression [12], $\tau_\mathrm{v} = \eta/G = 36$ s $= 6.3\,\tau_\mathrm{B}$. The fixed and fitted parameters are summarized in Tab. SM-1.

Also for the small particles, $R$, $\phi$ and $\dot{\gamma}$ are given through the sample composition and experimental conditions. Concerning the conditions, it is important to note that the sample containing large particles with $\phi = 0.565$ shows a similar (scaled) rheological response as the sample containing small particles with $\phi = 0.570$ and for comparable Peclet numbers, $Pe_0 = 6\pi\eta_\mathrm{s}\dot{\gamma}R^3/k_\mathrm{B}T$, i.e. $\dot{\gamma} = 0.0028$ $\mathrm{s}^{-1}$ and $\dot{\gamma} = 0.23$ $\mathrm{s}^{-1}$, respectively. The slightly larger $\phi$ is attributed to uncertainties in the volume fraction [2] and the different polydispersities, $\sigma_{\mathrm{R},1} > \sigma_{\mathrm{R},2}$. Thus the samples with $R_2 = 780$ nm, $\phi = 0.565$, $\dot{\gamma} = 0.0028$ $\mathrm{s}^{-1}$ and $R_1 = 150$ nm, $\phi_0 = 0.570$, $\dot{\gamma}_0 = 0.23$ $\mathrm{s}^{-1}$, respectively, correspond to each other and the latter, i.e. $\phi_0$ and $\dot{\gamma}_0$, will be used as reference conditions and exploited in the fitting procedure as described below.

The small particles cannot be resolved by confocal microscopy and thus $n_0$, $c$ and $\xi$ cannot be determined directly and $\kappa$ cannot be determined through $g(r)$. We assume that $n_0 = 10.7$ and $c = 0$ also hold for the small particles under all conditions. Furthermore, $\kappa$ can be determined through the initial slope of $\sigma_\mathrm{tot}(\gamma)$. Since $\sigma_\mathrm{tot}(\gamma)/\sigma_\mathrm{tot}(\gamma{\to}\infty)$ seems independent of $\phi$ in the investigated range of $\phi$ (Fig. 3b, inset), the $\phi$ dependence of $\kappa$ can be deduced from the constant initial slope, i.e. from $G/\sigma_\mathrm{tot}(\gamma{\to}\infty) = \mathrm{const.}$ Hence

$$\kappa(\phi) = \frac{\eta(\phi)\phi_0}{\eta_0\phi}\,\kappa_0 \qquad \text{(SM-4)}$$

with the reference condition $\phi_0 = 0.570$ and the corresponding $\eta_0 = 4.15$ Pa s (see below). For this condition we assume that $\kappa_0 = 50\,k_\mathrm{B}T/R_1^2$ as for the corresponding conditions for the large particles. This puts a helpful constraint on the values of $\kappa(\phi,\dot{\gamma})$ and hence only for each additional $\dot{\gamma}$ one value of $\kappa$ has to be determined from the initial slope of $\sigma_\mathrm{tot}(\gamma)$. The absence of a $\phi$ dependence of $\sigma_\mathrm{tot}(\gamma)/\sigma_\mathrm{tot}(\gamma{\to}\infty)$ also implies that $\xi$ is independent of $\phi$. Furthermore, we assume that $\xi(\dot{\gamma}{=}0.23\mathrm{s}^{-1})$ of the small particles equals $\xi(\dot{\gamma}{=}0.0028\mathrm{s}^{-1})$ of the large particles since these two conditions correspond to each other and hence $\xi(\dot{\gamma}{=}0.23\mathrm{s}^{-1})$ is fixed and only one $\xi$ for each additional $\dot{\gamma}$, i.e. in total three values for all data sets, need to be fitted.

The parameters describing the viscous contribution, $\eta$, $\tau_\mathrm{v}$ and $\beta$, are independently determined or related to the values for the large particles. The viscosity $\eta$ again is determined from the steady-state value of the total stress, $\eta = \sigma_\mathrm{tot}(\gamma{\to}\infty)/\dot{\gamma}$ for all $\phi$ and $\dot{\gamma}$. The exponent $\beta$ is assumed to be independent of $\phi$ and $\dot{\gamma}$ and is inferred from the value determined for the large particles, $\beta = 4.6$. The viscous time scale $\tau_\mathrm{v}$ is also linked to the value for the large particles. For the corresponding conditions, $\phi_0 = 0.570$ and $\dot{\gamma}_0 = 0.23$ $\mathrm{s}^{-1}$, the viscous time scale is scaled by the imposed shear rates, i.e. $\tau_{\mathrm{v},0} = \tau_{\mathrm{v,L}}(\dot{\gamma}_\mathrm{L}/\dot{\gamma}_0)$, where the index L refers to the large particles. Maxwell's expression, $\tau_\mathrm{v} = \eta/G$ [12], suggests

$$\tau_\mathrm{v}(\phi,\dot{\gamma}) = \frac{\eta(\phi,\dot{\gamma})\,\kappa_0\,\phi_0}{\eta_0\,\kappa(\dot{\gamma})\,\phi}\,\tau_{\mathrm{v},0} = \frac{\eta(\phi,\dot{\gamma})\,\kappa_0\,\phi_0\,\dot{\gamma}_\mathrm{L}}{\eta_0\,\kappa(\dot{\gamma})\,\phi\,\dot{\gamma}_0}\,\tau_{\mathrm{v,L}} \quad . \qquad \text{(SM-5)}$$

Hence, $\tau_\mathrm{v}(\phi,\dot{\gamma})$ can be linked to the values of the large particles for all conditions and hence can be fixed and does not need to be fitted.

For the small particles, therefore, the transient total stress $\sigma_\mathrm{tot}(\gamma)$ for all volume fractions $\phi$ and shear rates $\dot{\gamma}$ investigated (Fig. SM-2b–e) can be fitted by Eq. SM-3 and only three free parameters, namely the three values of $\xi$ for the additional $\dot{\gamma}$. The values of all other parameters are independently determined and/or linked to the values of the large particles as described above. The fixed and fitted parameters are summarized in Tab. SM-2. Under all conditions, $\sigma_\mathrm{tot}(\gamma)$ is well described by our model. Only at the transition from elastic to viscous behavior a spurious dip occurs at $\gamma \approx \xi$, where $\xi$ depends on $\dot{\gamma}$. This dip is due to the abrupt transition to the constant value $\sigma_\mathrm{el}(\gamma{\geq}\xi)$ mentioned above. As also discussed above, this abrupt transition is unphysical and hence should be avoided. However, this would require additional free parameters or some assumptions which we prefer not to introduce.

The fixed and fitted as well as a few deduced parameters (Tab. SM-2) are compared to previous findings. The

TABLE SM-2. Dependence of the fixed and fitted as well as some deduced parameters on the volume fraction $\phi$ and the applied shear rate $\dot{\gamma}$ for the small particles (radius $R_1 = 150$ nm); decay parameter $\xi$, effective spring constant $\kappa$, viscosity $\eta$ and the viscous time scale $\tau_\mathrm{v}$ as well as the deduced parameters shear modulus $G$ and activation volume $V^*$. Only the three bold values of $\xi$ were fitted, all other values were determined independently as explained in the text. Furthermore, the initial number of long-lived neighbors $n_0 = 10.7$, the first order term $c = 0$ and stretching exponent $\beta = 4.6$ were fixed for all conditions.

| $\phi$ [1] | $\dot{\gamma}$ $[\mathrm{s}^{-1}]$ | $\xi$ [1] | $\kappa$ $\left[\frac{k_\mathrm{B}T}{R_1^2}\right]$ | $\eta/\eta_\mathrm{s}$ [1000] | $\tau_\mathrm{v}$ $[\tau_\mathrm{B}]$ | $G$ $\left[\frac{k_\mathrm{B}T}{R_1^3}\right]$ | $V^*$ $\left[\frac{4\pi}{3}R_1^3\right]$ |
|---|---|---|---|---|---|---|---|
| 0.570 | 0.069 | **0.27** | 33 | 2.25 | 57 | 8.3 | 0.326 |
| 0.570 | 0.23 | 0.31 | 50 | 1.15 | 19 | 12.5 | 0.198 |
| 0.570 | 0.69 | **0.40** | 55 | 0.55 | 8.4 | 13.7 | 0.161 |
| 0.570 | 2.07 | **0.51** | 69 | 0.31 | 3.7 | 17.4 | 0.115 |
| 0.580 | 0.069 | 0.27 | 94 | 6.56 | 57 | 24.2 | 0.127 |
| 0.580 | 0.23 | 0.31 | 114 | 2.69 | 19 | 29.1 | 0.095 |
| 0.580 | 0.69 | 0.40 | 128 | 1.31 | 8.4 | 32.7 | 0.077 |
| 0.580 | 2.07 | 0.51 | 150 | 0.68 | 3.7 | 38.5 | 0.059 |
| 0.600 | 0.23 | 0.31 | 318 | 7.81 | 19 | 84.3 | 0.037 |
| 0.600 | 0.69 | 0.40 | 331 | 3.50 | 8.4 | 87.7 | 0.033 |

decay parameter $\xi$ increases with $\dot{\gamma}$, as previously predicted [13]. This reflects the increasing contribution of shear compared to Brownian motion which results in the dominance of affine motions and hence particles remain neighbors for larger strains. The spring constant $\kappa$, and hence the shear modulus $G$, increase with $\phi$ due to the tightening of the cages. Their increase with $\dot{\gamma}$ results from the increasing effect of shear compared to structural cage relaxations and hence a decreasing entropic elasticity, in agreement with previous findings and theoretical predictions [14, 15]. The obtained $\eta(\phi, \dot{\gamma})$ increases with $\phi$ and decreases with $\dot{\gamma}$, in agreement with previous flow curve measurements [16–18]. These values indicate an active volume $V^* = (k_\mathrm{B}T/G)\ln(\eta/\eta_\mathrm{s})$ [12] of a fraction of the particle volume that decreases with $\phi$ and $\dot{\gamma}$, which is attributed to the increasing space filling and effect of shear. While $\tau_\mathrm{v}$ is independent of $\phi$, it was found to decrease with $\dot{\gamma}$ according to $\tau_\mathrm{v} \sim \dot{\gamma}^{-0.80}$. This decrease is due to the increasing fluidization of the system. The relaxation time $\tau_\mathrm{v}$ is expected to be inversely proportional to the diffusion coefficient, $D(\dot{\gamma}) \sim \tau_\mathrm{v}^{-1} \sim \dot{\gamma}^{0.80}$. This can be compared to previous findings $D(\dot{\gamma}) \sim \dot{\gamma}^{0.8}$ [6] and $D(\dot{\gamma}) \sim \dot{\gamma}^{1}$ [19].


[1] C. P. Royall, W. C. K. Poon, and E. R. Weeks, Soft Matter **9**, 17 (2013).

[2] W. C. K. Poon, E. R. Weeks, and C. P. Royall, Soft Matter, **8**, 21 (2012).

[3] P. N. Pusey and W. van Megen, Phys. Rev. Lett. **59**, 2083 (1987).

[4] A. Yethiraj and A. Van Blaaderen, Nature **421**, 513 (2003).

[5] M. Laurati, K. J. Mutch, N. Koumakis, J. Zausch, C. P. Amann, A. B. Schofield, G. Petekidis, J. F. Brady, J. Horbach, M. Fuchs, and S. U. Egelhaaf, J. Phys.: Condens. Matter **24**, 464104 (2012).

[6] R. Besseling, E. R. Weeks, A. B. Schofield, and W. C. K. Poon, Phys. Rev. Lett. **99**, 028301 (2007).

[7] J. Zausch, J. Horbach, M. Laurati, S. U. Egelhaaf, J. M. Brader, T. Voigtmann, and M. Fuchs, J. Phys.: Condens. Matter **20**, 404210 (2008).

[8] J. C. Crocker and D. G. Grier, J. Coll. Interface Sci. **179**, 298 (1996).

[9] M. C. Jenkins and S. U. Egelhaaf, Adv. Coll. Interf. Sci. **136**, 65 (2008).

[10] J.-P. Hansen and I. R. MacDonald, *Theory of Simple Liquids* (Academic Press, London, 2005).

[11] K. S. Schweizer, E. J. Saltzmann, J. Chem. Phys. **119**, 1181 (2003).

[12] J. C. Dyre, J. Non-Cryst. Solids **235–237**, 142 (1998).

[13] A. Zaccone, P. Schall, and E. M. Terentjev, Phys. Rev. B **90**, 140203(R) (2014).

[14] K. S. Schweizer and E. J. Saltzmann, J. Chem. Phys. **119**, 1181 (2003).

[15] N. Koumakis, A. Pamvouxoglou, A. S. Poulos, and G. Petekidis, Soft Matter **8**, 4271 (2012).

[16] G. Petekidis, D. Vlassopoulos, and P. N. Pusey, J. Phys.: Condens. Matter **16**, S3955 (2004).

[17] M. Fuchs and M. Ballauff, J. Chem. Phys. **122**, 094707 (2005).

[18] F. Varnik and O. Henrich, Phys. Rev. B **73**, 174209 (2006).

[19] K. Miyazaki, H. M. Wyss, D. A. Weitz, and D. R. Reichman, Europhys. Lett. **75**, 915 (2006).
